# Supplementary material for: Relational Multi-Task Learning: Modeling Relations between Data and Tasks
Source: arXiv:2303.07666 source file (2023-03-14)
Supplement: Supplementary file 1 [file main_appendix.tex]

\documentclass{article}

\PassOptionsToPackage{numbers, compress}{natbib}
\usepackage{neurips_2021}
\input{math_macro}

\usepackage[utf8]{inputenc} %
\usepackage[T1]{fontenc}    %
\usepackage[colorlinks=true,citecolor=green]{hyperref}
\usepackage{url}            %
\usepackage{booktabs}       %
\usepackage{amsfonts}       %
\usepackage{nicefrac}       %
\usepackage{microtype}      %
\usepackage{xcolor}         %
\usepackage{graphicx}
\usepackage{float}
\usepackage{scalerel,amssymb}
\usepackage{algorithm}
\usepackage[noend]{algpseudocode}

\def\shownotes{1}  %
\ifnum\shownotes=1
\newcommand{\authnote}[2]{[#1: #2]}
\else
\newcommand{\authnote}[2]{}
\fi

\usepackage{multirow}
\usepackage{multicol}
\usepackage{tabularx}

\usepackage{xspace}
\usepackage{caption}
\usepackage{graphicx}
\usepackage{booktabs}

\newcommand{\cut}[1]{}

\usepackage{titlesec}
\titlespacing\section{0pt}{4pt plus 2pt minus 1pt}{4pt plus 2pt minus 1pt}
\titlespacing\subsection{0pt}{3pt plus 2pt minus 1pt}{3pt plus 2pt minus 1pt}

\title{Appendix for ``Relational Multi-Task Learning:\\
Modeling Relations between Data and Tasks''}

\author{%
  David S.~Hippocampus\thanks{Use footnote for providing further information
    about author (webpage, alternative address)---\emph{not} for acknowledging
    funding agencies.} \\
  Department of Computer Science\\
  Cranberry-Lemon University\\
  Pittsburgh, PA 15213 \\
  \texttt{hippo@cs.cranberry-lemon.edu} \\
}

\begin{document}

\maketitle

\appendix

\input{070appendix}

\bibliography{main}
\bibliographystyle{unsrtnat}

\end{document}
